# Supplementary material for: Aligning coding sequences with frameshift extension penalties
Source: arXiv:1610.08809 source file (2017-04-13)
Supplement: Supplementary file 1 [file additional_file_1.tex]

\documentclass[11pt, a4paper]{article}

\usepackage{amssymb,xspace,amsmath,amsthm}
\usepackage[utf8]{inputenc}
\usepackage{bm}
\usepackage{url} 
\usepackage{color}
\usepackage{multirow}

\begin{document} 

\title{Additional file  -- Proof of Lemma1 \\
Aligning coding sequences with frameshift extension penalties
}
\author{Safa Jammali et al. \\
Department of Computer Science, Universit\'e de Sherbrooke,\\
Sherbrooke, QC, Canada \\
Email: safa.jammali@usherbrooke.ca}

\date{}
                      
\maketitle

Following the definitions and notations for frameshifts used in
[14], given an alignment between two CDS $A$ and $B$,
the set of \texttt{FSinit} codons of $A$ (resp. $B$) can be divided
into two sets. The set of \texttt{FSinit codons}
\texttt{caused by deletions (FS$^-$)} contains the
\texttt{FSinit} codons that are grouped in the alignment and are aligned
with at least one nucleotide and at least one gap symbol in the other CDS.
The set of \texttt{FSinit codons caused by insertions} \texttt{(FS$^+$)}
contains all the codons that are not grouped in the alignment.

\subsection*{Proof of Lemma 1}
  The principle of the proof is
  similar to the one for the alignment of non-coding sequences.
  For each of the cases 1, 2, 3 and 4 of the Lemma, the score $D(i,j)$ is the
  maximum score of all possible alignment configurations that are considered
  for this case. An illustration of the different configurations of
  alignment considered for the cases 1 and 2 is shown in Figure 2 of the
  main manuscript.

  For each case, we first consider three sub-cases depending on the
  configurations of the alignment of $A[i]$ and $B[j]$: (a) $A[i]$ and $B[j]$
  are aligned together, (b) $A[i]$ is aligned with a gap, (c) $B[j]$ is
  aligned with a gap.
    \begin{enumerate}
   \item {\bf If $i (mod~3) = 0$ and $j (mod~3) = 0$}, then $A[i]$ and $B[j]$ are
     the last nucleotides of two codons $A[i-2~..~i]$ and $B[j-2~..~j]$. There are
     three cases depending on the alignment of $A[i]$ and $B[j]$.
      \begin{enumerate}
      \item {\bf If $A[i]$ and $B[j]$ are aligned together}, there are four cases
        depending on whether $A[i-2~..~i]$ and $B[j-2~..~j]$ are grouped in
        the alignment or not.
        \begin{enumerate}
        \item {\bf If both $A[i-2~..~i]$ and $B[j-2~..~j]$ are grouped}, then
          $A[i-2~..~i]$ and $B[j-2~..~j]$  have to be aligned together and the
          score of the alignment is:\\
          1.  $s_{aa}(A[i-2~..~i],B[j-2~..~j]) + D(i-3,j-3)$
        \item {\bf If  $A[i-2~..~i]$ is grouped while  $B[j-2~..~j]$ is not grouped},
          then both $A[i-2~..~i]$ and $B[j-2~..~j]$ are FS codons ($A[i-2~..~i]$ is
          a FS$^-$ codon while $B[j-2~..~j]$ is a FS$^+$ codon). We add
          $2 * \texttt{fs\_open\_cost}$ to the score of the alignment and
          the alignment of the nucleotides of the two FS codons can be scored
          independently using the scoring function $s_{an}$.
         There are two cases depending on the number of  nucleotides from
          $B[j-2~..~j]$ that are aligned with $A[i-2~..~i]$, two or one:
            \begin{enumerate}
            \item {\bf If  $A[i-2~..~i]$ is aligned with two nucleotides}, then these
              nucleotides are $B[j-1]$ and $B[j]$.
              There are two cases depending on the alignment of the nucleotide
              $B[j-1]$ with $A[i-1]$ or $A[i-2]$:\\
              2. $s_{an}(A[i],B[j]) + s_{an}(A[i-1],B[j-1]) + D(i-3,j-2) + 2 * \texttt{fs\_open\_cost}$\\
              3. $s_{an}(A[i],B[j]) + s_{an}(A[i-2],B[j-1]) + D(i-3,j-2) + 2 * \texttt{fs\_open\_cost}$
            \item {\bf If  $A[i-2~..~i]$ is aligned with one nucleotide},  then
              this single nucleotide is $B[j]$ and the score of the alignment is:\\
             4. $s_{an}(A[i],B[j]) + D(i-3,j-1) + 2 * \texttt{fs\_open\_cost}$
            \end{enumerate}
          \item  {\bf If  $A[i-2~..~i]$ is not grouped while $B[j-2~..~j]$ is grouped},
            there are three cases that are symmetric to the three cases from
            (a)ii.:\\
            5. $s_{an}(A[i],B[j]) + s_{an}(A[i-1],B[j-1]) + D(i-2,j-3) + 2 * \texttt{fs\_open\_cost}$\\
            6. $s_{an}(A[i],B[j]) + s_{an}(A[i-1],B[j-2]) + D(i-2,j-3) + 2 * \texttt{fs\_open\_cost}$\\
            7. $s_{an}(A[i],B[j]) + D(i-1,j-3) + 2 * \texttt{fs\_open\_cost}$
          \item {\bf If both $A[i-2~..~i]$ and $B[j-2~..~j]$ are not grouped}, then again
        both $A[i-2~..~i]$ and $B[j-2~..~j]$ are FS codons (both are FS$^+$ codons):\\
        8. $s_{an}(A[i],B[j]) + D(i-1,j-1) + 2 * \texttt{fs\_open\_cost}$\\
        \end{enumerate}
        
      \item {\bf If $A[i]$ is aligned with a gap}, then the codon  $A[i-2~..~i]$
        is a FS codon (FS$^-$ or FS$^+$). We must add $\texttt{fs\_open\_cost}$
        to the score of
        the alignment. There are two cases depending on whether
        $A[i-2~..~i]$ is grouped in the alignment or not.
        \begin{enumerate}
        \item {\bf If $A[i-2~..~i]$ is grouped}, then there are three cases depending
          on the number of  nucleotides from $B[j-2~..~j]$ that are aligned
          with $A[i-2~..~i]$, two, one, or zero.
            \begin{enumerate}
            \item {\bf If  $A[i-2~..~i]$ is aligned with two nucleotides}, then
              these
              nucleotides are $B[j-1]$ and $B[j]$. The score of the alignment is:\\
              9. $\frac{s_{an}(A[i-1],B[j])}{2} + \frac{s_{an}(A[i-2],B[j-1])}{2} + D_F(i-3,j-2) + \texttt{fs\_open\_cost}$
            \item {\bf If  $A[i-2~..~i]$ is aligned with one nucleotide}, then this
              single nucleotide is $B[j]$. There two cases depending on
              the alignment of the nucleotide $B[j]$ with $A[i-1]$ or $A[i-2]$:\\
              10. $s_{an}(A[i-1],B[j]) + D(i-3,j-1) + 2 * \texttt{fs\_open\_cost}$\\
              11. $\frac{s_{an}(A[i-2],B[j])}{2} + D_F(i-3,j-1) + \texttt{fs\_open\_cost}$
            \item {\bf If $A[i-2~..~i]$ is aligned with zero nucleotide}, then
              the codon
        $A[i-2~..~i]$ is entirely deleted. The score of the alignment is: \\
              12. $\texttt{gap\_cost} + D(i-3,j)$ 
            \end{enumerate}
          \item  {\bf If $A[i-2~..~i]$ is not grouped}, then the codon $A[i-2~..~i]$
            is a FS$^+$ codon and the score of the alignment is:\\
        13. $D(i-1,j) + \texttt{fs\_open\_cost}$\\  
        \end{enumerate}

      \item {\bf If $B[i]$ is aligned with a gap}, there are fives cases that
        are symmetric
        to the five cases from (b):\\
        14. $\frac{s_{an}(A[i],B[j-1])}{2} + \frac{s_{an}(A[i-1],B[j-2])}{2} + D_F(i-2,j-3) + \texttt{fs\_open\_cost}$\\
        15. $s_{an}(A[i],B[j-1]) + D(i-1,j-3) + 2 * \texttt{fs\_open\_cost}$\\  
        16. $\frac{s_{an}(A[i],B[j-2])}{2} + D_F(i-1,j-3) + \texttt{fs\_open\_cost}$\\
         17. $\texttt{gap\_cost} + D(i,j-3)$\\
         18. $D(i,j-1) + \texttt{fs\_open\_cost}$\\  
      \end{enumerate}

    \item {\bf If $i (mod~3) = 0$ and $j (mod~3) \neq 0$}, then $A[i]$ is the
      last nucleotide of a codon $A[i-2~..~i]$ and $B[j]$ is not the last
      nucleotide of a codon. There are three cases depending on the alignment
      of $A[i]$ and $B[j]$.
      \begin{enumerate}
      \item {\bf If  $A[i]$ and $B[j]$ are aligned together},  there are
        two cases depending on whether $A[i-2~..~i]$  is grouped in the
        alignment or not.
        \begin{enumerate}
        \item {\bf If $A[i-2~..~i]$ is grouped}, there are three cases depending
          on the number of nucleotides from $B$ that are aligned with
          $A[i-2~..~i]$, three, two, or one:
          \begin{enumerate}
          \item  {\bf If  $A[i-2~..~i]$ is aligned with three nucleotides}, then
            these nucleotides are $B[j]$, $B[j-1]$ and $B[j-2]$. We are in
            the case of a FSext codon. The score of the alignment is
            then:\\      
          1. $\frac{s_{aa}(A[i-2~..~i],B[j-2~..~j])}{2} + D_F(i-3,j-3) + \texttt{fs\_extension\_cost}$ + $\frac{s_{an}(A[i],B[j])}{2} ~(+ \frac{s_{an}(A[i-1],B[j-1])}{2} ~if ~j-1 (mod~3) \neq 0)$
          \item {\bf If  $A[i-2~..~i]$ is aligned with two nucleotides}, then
            these nucleotides are $B[j]$ and $B[j-1]$. $A[i-2~..~i]$ is a FS$^-$
            codon. There are two cases
            depending of the alignment of $B[j-1]$ with $A[i-1]$ or $A[i-2]$.
            In both cases, if $j-1 (mod~3) = 0$, then $j-1$ is the last
            nucleotide of a codon. We should then make adjustments in order to
            account for the type of this codon (FS$^+$, or unknown type for now):\\      
          2. $s_{an}(A[i],B[j]) + s_{an}(A[i-1],B[j-1]) + D(i-3,j-2) + \texttt{fs\_open\_cost} ~(+ \texttt{fs\_open\_cost} ~if ~j-1 (mod~3) = 0)$\\
          3. $s_{an}(A[i],B[j]) + s_{an}(A[i-2],B[j-1]) + D_F(i-3,j-2) + \texttt{fs\_open\_cost} ~(- \frac{s_{an}(A[i-2],B[j-1])}{2} ~ if ~ j-1 (mod~3) = 0)$
        \item {\bf If  $A[i-2~..~i]$ is aligned with one nucleotide}, then
          $A[i-2~..~i]$ is a FS$^-$ codon. The score of the alignment is:\\      
          4. $s_{an}(A[i],B[j]) + D(i-3,j-1) + \texttt{fs\_open\_cost}$
          \end{enumerate}
        \item {\bf If $A[i-2~..~i]$ is not grouped}, then $A[i-2~..~i]$ is a
          FS$^+$ codon:\\
         5. $s_{an}(A[i],B[j]) + D(i-1,j-1) + \texttt{fs\_open\_cost}$
        \end{enumerate}
        
      \item {\bf If  $A[i]$ is aligned with a gap},  there are
        two cases depending on whether $A[i-2~..~i]$  is grouped in the
        alignment or not.
        \begin{enumerate}
        \item {\bf If $A[i-2~..~i]$ is grouped}, there are three cases depending
          on the number of nucleotides from $B$ that are aligned with
          $A[i-2~..~i]$, two, one, or zero.
          \begin{enumerate}
          \item {\bf If  $A[i-2~..~i]$ is aligned with two nucleotides}, then
            these nucleotides are $B[j]$ and $B[j-1]$. $A[i-2~..~i]$ is a
            FS$^-$ codon. If $j-1 (mod~3) = 0$, then $j-1$
            is the last nucleotide of a codon. We should make adjustments
            in order to account for the fact no type has yet been decided
            for this codon.\\      
         6. $ s_{an}(A[i-1],B[j]) + s_{an}(A[i-2],B[j-1]) + D_F(i-3,j-2) + \texttt{fs\_open\_cost} ~(- \frac{s_{an}(A[i-2],B[j-1])}{2} ~if ~j-1 (mod~3) = 0)$
          \item {\bf If  $A[i-2~..~i]$ is aligned with one nucleotide}, then
            this single nucleotide is $B[j]$.
            $A[i-2~..~i]$ is a FS$^-$ codon. There are two cases depending
            on the alignment of $B[j]$ with $A[i-1]$ or $A[i-2]$:\\      
         7. $s_{an}(A[i-1],B[j]) + D(i-3,j-1) + \texttt{fs\_open\_cost}$\\
         8. $s_{an}(A[i-2],B[j]) + D(i-3,j-1) + \texttt{fs\_open\_cost}$
       \item {\bf If $A[i-2~..~i]$ is aligned with zero nucleotide}, the codon
        $A[i-2~..~i]$ is entirely deleted:\\      
         9. $\texttt{gap\_cost} + D(i-3,j)$
          \end{enumerate}
        \item {\bf If $A[i-2~..~i]$ is not grouped}\\
         10. $D(i-1,j) + \texttt{fs\_open\_cost}$
       \end{enumerate}
      \item {\bf If  $B[j]$ is aligned with a gap}, then the score of the
        alignment is:\\
         11. $D(i,j-1)$\\
    \end{enumerate}

      \item {\bf If  $i (mod~3) \neq 0$ and $j (mod~3) = 0$}, the proof is
        symmetric to the previous proof for 2.\\
        
      \item {\bf If  $i (mod~3) \neq 0$ and $j (mod~3) \neq 0$}, there are
        three cases depending on the alignment of $A[i]$ and $B[j]$.
      \begin{enumerate}
      \item {\bf If  $A[i]$ and $B[j]$ are aligned together}, the score of the
        alignment is:\\
      1. $s_{an}(A[i],B[j]) + D(i-1,j-1)$
      \item {\bf If  $A[i]$ is aligned with a gap}, the score of the
        alignment is:\\
      2. $D(i-1,j)$
      \item {\bf If  $B[j]$ is aligned with a gap}, the score of the
        alignment is:\\
      3. $D(i,j-1)$    
      \end{enumerate}

  \end{enumerate}
\flushright
$\qed$
\end{document}
